# Supplementary material for: Automating Reasoning with Standpoint Logic via Nested Sequents
Source: arXiv:2205.02749 source file (2022-05-05)
Supplement: Supplementary file 1 [file appendix.tex]

\begin{customthm}{\ref{thm:soundness}}[Soundness]
If $\sprset \sep \nseq$ is derivable in $\nspv$, then $\sprset \sep \nseq$ is valid.
\end{customthm}

\begin{proof} We prove the remaining cases of the inductive step below.

$\disr$. The result immediately follows from the fact that the formula interpretation of the premise is identical to the formula interpretation of the conclusion.

$\conr$. Let us assume that $\Sigma_{1}$ is of the form $\phi \land \psi, \Sigma_{1}'$ with $\phi \land \psi$ the principal formula; all remaining cases are similar. Suppose that $\iota(\Gamma \vdash \Delta\{\phi \land \psi\}_{\pi_{1}}) := $
$$
\bigwedge \sprset \rightarrow \bigvee \Sigma_{0} \lor \spbox{s_{1}}(\phi \land \psi \lor \bigvee \Sigma_{1}')  \lor \bigvee_{2\leq i \leq n} \spbox{s_{i}}(\bigvee \Sigma_{i}) 
$$
is invalid. Then, there exists a standpoint model $\model := \langle \Pi, \sigma, \delta \rangle$ with a precisification $\pi$ falsifying the above formula. Consequently, $\model, \pi \not\models \spbox{s_{1}}(\phi \land \psi \lor \bigvee \Sigma_{1}')$, meaning that there exists a precisification $\pi' \in \sigma(s_{1})$ such that $\model, \pi' \not\models \phi$ or $\model, \pi' \not\models \psi$. The former case falsifies the left premise of $\conr$, and the latter falsifies the right premise.

$\nr{s}$. Let $s \in \spset$ and suppose that the following is invalid:
$$
\iota(\sprset \sar \nseq) := \bigwedge \sprset \rightarrow \bigvee\nseq
$$
Hence, there is a standpoint model $\model := \langle \Pi, \sigma, \delta \rangle$ with precisification $\pi$ such that $\model, \pi \not\models \iota(\sprset \sar \nseq)$.  By \dfn~\ref{def:standpoint-models}, we know that  $\sigma(s) \neq \emptyset$ for every $s \in \spset$. %, implying that for some $\pi' \in \Pi$, $\pi' \in \sigma(s)$. 
It follows that $\model, \pi \models \spdia{s} \top$, which entails that $\model, \pi \not\models \spbox{s} \bot$, thus showing that the premise of $\nr{s}$ is
%$$ \iota(\sprset \sar \nseq, (s)[\emptyset]_{\pi'}) := \bigwedge \sprset \rightarrow \bigvee\nseq \lor \spbox{s} \bot $$
invalid.

$\spdiarii{s}$. Suppose that $s' = s_{n}$, $\pi = \pi_{n}$, $\Sigma = \Sigma_{n}$, $s' \sprel s$, and $\iota(\sprset \sep \nseq, (s')[\spdia{s} \phi, \Sigma]_{\pi}) :=$
$$
\bigwedge \sprset \rightarrow \bigvee \Sigma_{0} \lor \Big(\bigvee_{1\leq i \leq n-1}\!\!\!\!\!\!\! \spbox{s_{i}}(\bigvee \Sigma_{i})\Big) \lor \spbox{s'}(\spdia{s} \phi \lor \bigvee \Sigma)
$$
is invalid. Therefore, there is a standpoint model $\model := \langle \Pi, \sigma, \delta \rangle$ with $\pi \in \Pi$ such that $\model, \pi \not\models \spbox{s'}(\spdia{s} \phi \lor \bigvee \Sigma)$. This entails that there exists a precisification $\pi_{1} \in \sigma(s')$ such that $\model, \pi_{1} \not\models \spdia{s} \phi$ and $\model, \pi_{1} \not\models \bigvee \Sigma$, further implying that for every precisification $\pi_{2} \in \sigma(s)$, $\model, \pi_{2} \not\models \phi$. Since $s' \sprel s$ holds, $\sigma(s') \subseteq \sigma(s)$ by \lem~\ref{lem:sprel-implies-sharpening} and \dfn~\ref{def:semantic-clauses}, implying that $\model, \pi_{1} \not\models \phi$ as $\pi_{1} \in \sigma(s') \subseteq \sigma(s)$ and $\model, \pi_{2} \not\models \phi$ or every precisification $\pi_{2} \in \sigma(s)$, thus proving the premise invalid.

$\spdiar{*}$. We assume that $\Sigma_{1}$ is of the form $\spdia{\dst},\Sigma_{1}'$ with $\spdia{\dst}$ principal; all remaining cases are shown in a similar fashion. Furthermore, suppose that
 $\iota(\sprset \sep \nseq\{\spdia{*} \phi\}_{\pi}) :=$
$$
\bigwedge \sprset \rightarrow \bigvee \Sigma_{0} \lor \spbox{s_{1}}(\spdia{\dst} \phi \lor \bigvee \Sigma_{1}') \lor \Big(\bigvee_{2\leq i \leq n}\!\!\!\! \spbox{s_{i}}(\bigvee \Sigma_{i})\Big)
$$
is invalid. Hence, there exists a standpoint model $\model := \langle \Pi, \sigma, \delta \rangle$ with $\pi \in \Pi$ such that $\model, \pi \not\models \spbox{s_{1}}(\spdia{\dst} \phi \lor \bigvee \Sigma_{1}')$, implying that for some $\pi_{1} \in \sigma(s_1)$, $\model,\pi_{1} \not\models \spdia{\dst} \phi$. As $\dst$ is the universal standpoint (see~\dfn~\ref{def:logical-languages}), it follows by \dfn~\ref{def:standpoint-models} and~\ref{def:semantic-clauses} that for all $\pi_{2} \in \Pi$, $\model,\pi_{2} \not\models \phi$. Therefore, $\model, \pi \not\models \phi$, proving the premise invalid.
\end{proof}
